# Supplementary material for: Packing polydisperse colloids into crystals: when charge-dispersity matters
Source: arXiv:1909.02774 ancillary file (2020-01-17)
Supplement: Supplementary file 1 [file Supplementary_Material.pdf]

# Supplemental material for: Packing polydisperse colloids into crystals: when charge-dispersity matters

Guillaume Bareigts,<sup>1</sup> Pree-Cha Kiatkirakajorn,<sup>2</sup> Joaquim Li,<sup>3</sup> Robert Botet,<sup>4</sup>  
Michael Sztucki,<sup>5</sup> Bernard Cabane,<sup>3</sup> Lucas Goehring,<sup>6,\*</sup> and Christophe Labbez<sup>1,†</sup>

<sup>1</sup>*ICB, CNRS UMR 6303, Univ. Bourgogne Franche-Comté, 21000 Dijon, France*

<sup>2</sup>*Max Planck Institute for Dynamics and Self-Organisation (MPIDS), Göttingen 37077, Germany*

<sup>3</sup>*LCMD, CNRS UMR 8231, ESPCI, 10 rue Vauquelin, 75231 Paris Cedex 05, France*

<sup>4</sup>*Physique des Solides, CNRS UMR 8502, Univ Paris-Sud, F-91405 Orsay, France*

<sup>5</sup>*ESRF-The European Synchrotron, CS40220, 38043 Grenoble Cedex 9, France*

<sup>6</sup>*School of Science and Technology, Nottingham Trent University, Nottingham, NG11 8NS, UK*

(Dated: January 17, 2020)

## CONTENTS

|                                                          |   |
|----------------------------------------------------------|---|
| S1. Size distribution of the TM50 silica dispersion      | 1 |
| S2. Interdiffusion experiments                           | 2 |
| S3. Experimental calibration and number densities        | 2 |
| S4. Model and simulation details                         | 2 |
| S5. Charge and interaction polydispersity                | 4 |
| S6. Convergence and equilibrium state of the simulations | 4 |
| S7. Simulation snapshots at phase coexistence            | 5 |
| S8. Phase composition and polydispersity                 | 5 |
| S9. Lattice simulation description and results           | 6 |
| S10. Characterisation of liquid and glass phases         | 8 |
| References                                               | 9 |

## S1. SIZE DISTRIBUTION OF THE TM50 SILICA DISPERSION

The size distribution of the industrially produced TM50 silica nanoparticle dispersion was estimated by numerical inversion of small-angle x-ray scattering data described elsewhere [1]. The experimental SAXS data were obtained from measurements carried out on the ID02 instrument at the European Synchrotron Radiation Facility in Grenoble, France. The wavelength of the X-rays was 0.1 nm, and the  $q$ -range was  $0.012 - 4.7 \text{ nm}^{-1}$ . The TM50 colloidal dispersion was diluted to a volume fraction  $\phi = 0.1 \%$  in mass.

The experimental radius distribution of TM50 particles was found to extend over the range  $10.0 - 17.3 \text{ nm}$ .

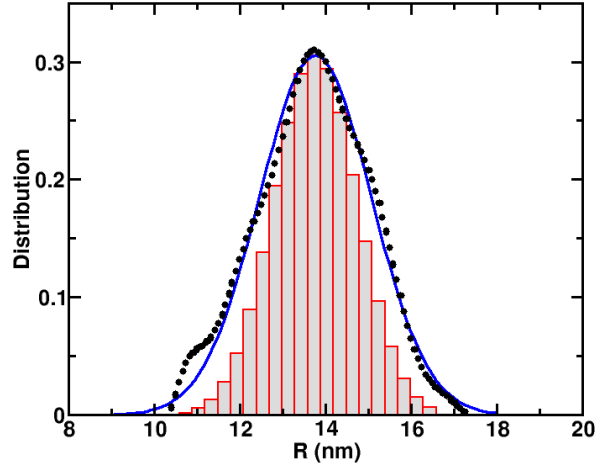

FIG. S1. Radius distribution,  $f(r)$ , of the TM50 silica nanoparticle dispersions including: experimental distribution obtained from SAXS data (black circles); best-fit curve of a continuous normal distribution, average radius  $13.75 \text{ nm}$  and polydispersity  $9.5\%$  (blue continuous curve); and discrete distribution made of 21 bins used in the numerical simulations, average radius  $13.75 \text{ nm}$  and polydispersity  $7\%$  (red histogram).

It is shown in Fig. S1 (black circles) and compared with the best-fit normal distribution with average radius  $\bar{R} = 13.75 \text{ nm}$  and polydispersity  $9.5\%$  (blue curve). The polydispersity is conventionally defined as the ratio between the standard deviation and the average value of the distribution. The distribution of the TM50 colloidal dispersion and the parameters of the distribution agree well with the conclusions of Ref. 2.

In the simulations, we used a discretized radius distribution made of 21 regular particle bins whose radii vary linearly between  $10.725 \text{ nm}$  and  $16.725 \text{ nm}$ . The same  $\bar{R}$  as, but somewhat lower polydispersity  $\delta = 7\%$  than, measured was used. This distribution is represented in Fig. S1 as the discrete distribution (red histogram).

\* lucas.goehring@ntu.ac.uk

† Christophe.labbez@u-bourgogne.fr

## S2. INTERDIFFUSION EXPERIMENTS

Samples of Ludox TM50 were dialysed against aqueous solutions of pH 9 (by addition of NaOH) and various concentrations of NaCl and PEG, as in the main text. A capillary tube ( $\sim 7$  cm long, 1 mm diameter) was carefully filled with two selected dispersions pipetted respectively into the bottom, then top half of the tube (with the heavier, higher density dispersion at the bottom). This created an initially sharp interface between dispersions of different volume fractions, but otherwise identical properties. A series of such capillary tubes were prepared, sealed and their samples were allowed to age, prior to scanning at ESRF. This allowed the dispersions to inter-diffuse, creating a continuous gradient in volume fractions. X-ray spectra were gathered at intervals (typically  $100 \mu\text{m}$ ) along the tubes, and scattering peaks used to identify the phases present at each position. Volume fractions were inferred from the location of the smallest- $q$  peak (or the broad first liquid-like peak of the glass samples), as described in Section S3. Some data are missing due to the presence of a sample holder, which blocked the beam at certain positions. However, a small but measurable jump in volume fraction between the crystal and jammed states was seen in all samples (see Fig. S2). The samples reported here for 5 mM initially contained dispersions with  $\phi = 0.190$  and  $\phi = 0.317$ , and were repeated for samples of age 5, 8, 15 and 23 days, with the location of the fcc/bcc/glass phase boundaries consistent to within  $\pm 0.5\%$ . A single experiment was tested at 10 mM, with an interface between  $\phi = 0.178$  and  $\phi = 0.349$  prepared 5 days before scanning.

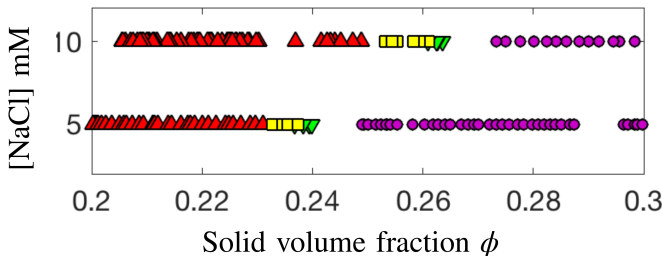

FIG. S2. Phases observed in interdiffusion experiments at steady state versus local particle volume fraction. When compared with Fig. 3 of the main text one can notice that the phase sequence fcc, fcc-bcc and bcc for increasing  $\phi$  is preserved. However, the transitions do not appear at the same  $\phi$  positions, most probably due to the density gradient of the colloids.

## S3. EXPERIMENTAL CALIBRATION AND NUMBER DENSITIES

The average solid volume fractions,  $\phi$ , of all experimental samples were measured by weighing sub-samples before and after drying in an oven overnight at  $120^\circ\text{C}$ ,

following the methods in Refs. [3, 4]. From these data we produced calibration curves. For the bcc and fcc crystals the positions  $q_{hkl}(\phi)$  of the scattering peaks from the  $(hkl)$  planes vary with volume fraction, and were used as calibrations for the inter-diffusion experiments. The position of any such peak scales inversely to the distance between the crystal planes, so  $\phi \sim q_{hkl}^3$ . The calibration curves for the fcc and bcc data are shown in Figure S3(a), based on the smallest- $q$  peak: (110) for bcc and (111) for fcc. For the high- $\phi$  glass phase, we measured the position of the first liquid-like peak, as in Ref. [3]. As shown in Fig. S3(a), the glass phase also follows the empirical relationship  $\phi \sim q_{peak}^3$ , and a fit to this data was used to infer  $\phi$  for the glass phase of the inter-diffusion experiments. Additionally, the crystal structure allows us to compare the particle number density of the various phases (although the actual volume fraction in each phase cannot be determined absolutely, if there is any fractionation). For this, we calculate the number density of the fcc phase as

$$N_{fcc} = \frac{q_{111}^3}{6\sqrt{3}\pi^3}, \quad (\text{S1})$$

for the bcc phase as

$$N_{bcc} = \frac{q_{110}^3}{8\sqrt{2}\pi^3}, \quad (\text{S2})$$

and for the total, or bulk, sample as

$$N_0 = \frac{3\phi}{4\pi R^3}. \quad (\text{S3})$$

As is shown in Fig. S2(b) the experimentally determined number densities in the two crystal phases are consistent with each other, and with the system-wide number density, to within experimental error.

## S4. MODEL AND SIMULATION DETAILS

The silica dispersion was modeled at the scale of the colloids with a multi-component model (MCM) for titratable polydisperse colloids detailed elsewhere [5]. In brief, within the MCM the colloids are defined by their radius  $R_i$  and renormalized charge number  $Z_i^*$  and interact through density-dependent effective hard core Yukawa pair potentials,

$$\beta w_{ij}^*(r) = \lambda_B Z_i^* Z_j^* f_i f_j \frac{\exp(-\kappa^* r)}{r} \quad (\text{S4})$$

when  $r > R_i + R_j$ , and

$$\beta w_{ij}^*(r) = \infty \quad (\text{S5})$$

otherwise.  $1/\kappa^*$  is the renormalized screening length,  $\lambda_B = 0.7105 \text{ nm}$  is the Bjerrum length and  $\beta = 1/k_B T$

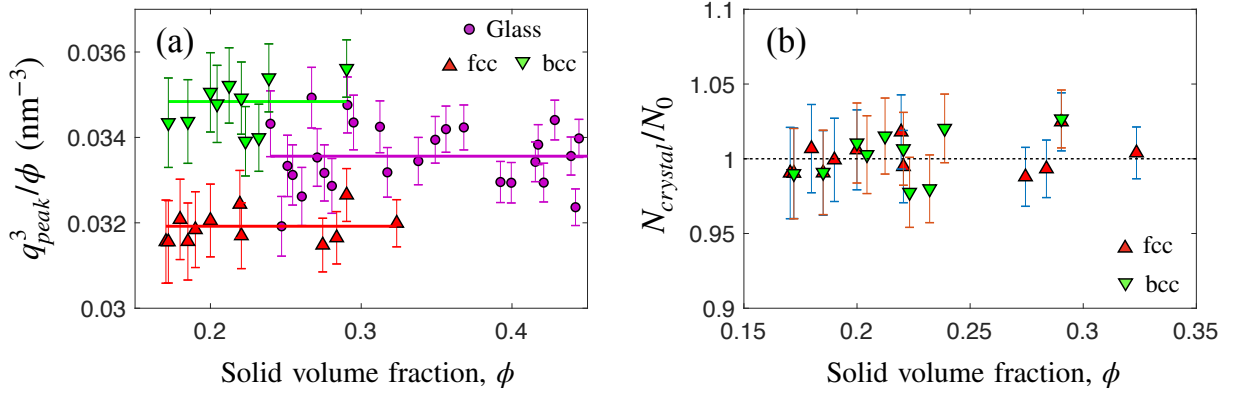

FIG. S3. Calibration and measurement of particle number densities. (a) To calibrate the inter-diffusion samples we fit the volume-fraction dependencies of the scattering peak positions of the various phases. For the glassy phase, this was the position of the first broad liquid-like peak, for the bcc phase the (110) peak, and for the fcc phase the (111) peak. (b) From the same crystal peak positions we also calculated the number densities of particles, which are consistent with the number densities inferred from the volume fraction of the bulk samples,  $N_0$ .

where  $k_B$  is the Boltzmann constant and  $T = 298$  K.  $f_i$  is a form factor which for an homogeneous silica sphere reads

$$f_i = \frac{\exp(-\kappa^* R_i)}{(1 + \kappa^* R_i)}. \quad (\text{S6})$$

Both  $Z_i^*$  and  $\kappa^*$  are density dependent due to the multi-body interactions arising in concentrated suspensions [6]. The set of  $Z_i^*(R_i, \phi)$  and  $\kappa^*(\phi)$  parameters were calculated using the polydisperse cell model (PCM) detailed in Ref. 5. The PCM further accounts for the charge regulation of the silica colloids arising from the pH dependent ionization of their surface silanol groups [7, 8], i.e.  $\text{Si-OH} \rightleftharpoons \text{Si-O}^- + \text{H}^+$ . The latter was modeled by a one pK Stern model parametrized with an independent experimental data set [9]. The details of the PCM used are described elsewhere [5]. The source code for the PCM employed, along with examples, are available at: <https://github.com/guibar64/polypbren>.

The so-defined MCM for silica suspensions only depends on well defined experimental quantities that is the pH and  $c_s$  of the bulk solution and the particle size distribution. It is thus free of adjustable parameters.

The MCM was solved with “in-house” Monte Carlo simulations in the NVT and NPT ensembles which, combined with a swap move [10], allow for the efficiently sampling of phase space up to high  $\phi$  [11]. The probability of swap moves was set to 0.3. The simulations were carried out in a cubic box with periodic boundary conditions and the minimum image convention. Simulations were performed with  $N = 19991$ , unless otherwise stated. A spherical cutoff of radius  $r_c$  was applied to the pair potential.  $r_c$  was set according to the interactions between the largest particles such that  $\beta u(r_c) \leq 0.1$ . A tail correction was applied to the total calculated energy. Simulations were further accelerated with the use of a cell decomposition [12]. Up to several tens of million of

MC cycles (1 MC cycle =  $N$  MC moves) for equilibration were used. Production runs lasted for  $10^5$  MC cycles.

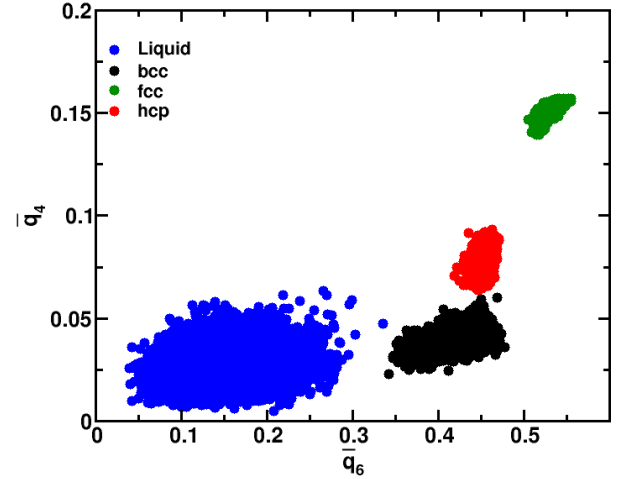

FIG. S4. Mean bond order parameter map of CS particles in various (thermalized) crystalline phases and in the fluid phase.

The mean local bond order parameters  $\bar{q}_6$  and  $\bar{q}_4$ , introduced and detailed by Lechner et al. [13], were used to analyze the obtained structures. As illustrated in Fig. S4(a), they allow for accurate discrimination between the phases of interest in this study, namely the fluid as well as the bcc, hcp and fcc solid phases. Note that we used only the nearest neighbors in the calculation of  $q_{lm}(i)$ .

The equation of state (EoS) was calculated by employing the analytical correction term (volume term) derived by Boon et al. [6], which, when added to the usual virial pressure of the MCM,  $P_{MCM}$ , has been shown to provide a very good approximation of the EoS calculated at the level of the full primitive model. The EoS defined as such

reads

$$\Pi_{EoS} = P_{MCM} + kT \frac{\kappa^{*2}}{8\pi l_B} \left( 1 - \left( \frac{\kappa}{\kappa^*} \right)^2 \right)^2 \quad (S7)$$

where  $\kappa$  is the inverse screening length of the bulk solution.

## S5. CHARGE AND INTERACTION POLYDISPERSITY

As for the size polydispersity, the charge polydispersity is defined as the ratio of its standard deviation to its mean value. The interaction polydispersity can be defined in the same way and is independent of the particle separation by virtue of the functional form of the Yukawa potential, Eq. S4. At a given separation  $r$ , size and charge distribution, the mean value of the Yukawa potentials can be defined as

$$\overline{\beta w^*(r)} = \lambda_D \frac{\exp(-\kappa r)}{r} \frac{1}{N} \sum_{i=1}^{N-1} \sum_{j=i+1}^N f_i f_j Z_i^* Z_j^* \quad (S8)$$

and its standard deviation as

$$SD(w^*(r)) = \lambda_D \frac{\exp(-\kappa r)}{r} \sqrt{\frac{1}{N-1} \sum_{i=1}^{N-1} \sum_{j=i+1}^N \left( f_i f_j Z_i^* Z_j^* - \frac{1}{N} \sum_{i=1}^{N-1} \sum_{j=i+1}^N f_i f_j Z_i^* Z_j^* \right)^2}. \quad (S9)$$

The interaction polydispersity is then given by

$$\lambda_{w^*} = \frac{\sqrt{\frac{1}{N-1} \sum_{i=1}^{N-1} \sum_{j=i+1}^N \left( f_i f_j Z_i^* Z_j^* - \frac{1}{N} \sum_{i=1}^{N-1} \sum_{j=i+1}^N f_i f_j Z_i^* Z_j^* \right)^2}}{\frac{1}{N} \sum_{i=1}^{N-1} \sum_{j=i+1}^N f_i f_j Z_i^* Z_j^*}. \quad (S10)$$

## S6. CONVERGENCE AND EQUILIBRIUM STATE OF THE SIMULATIONS

As a check of the consistency and equilibration of our simulation results, in the region where crystals were observed, we repeated some of the  $c_s - \phi$  state points with about 4000 and 40 000 particles. As it can be seen in Figure S5, the fraction of the various solid phases is very well reproduced when the system size is increased from 20 000 to 40 000 particles. In contrast, we found that simulations with only 4000 particles resulted in large variations in the relative fractions of the solid phases. This indicates that the correlation length is very large and that caution should be taken with the choice of the system size. We are working in the limit where system size effects are minimised.

Although pragmatic and efficient in predicting the experimental observations, the MC simulations employed are limited in two senses: (i) the exact phase boundaries and coexistence regions of the equilibrium phase diagram are not accessible; and (ii) the fractionation, relaxation and density fluctuation of the system may be limited due to finite size and interfacial effects [14]. In the specific case of interest here, after noting that the fluid composition and the size polydispersity of the different phases formed are rather insensitive to the volume fraction, a

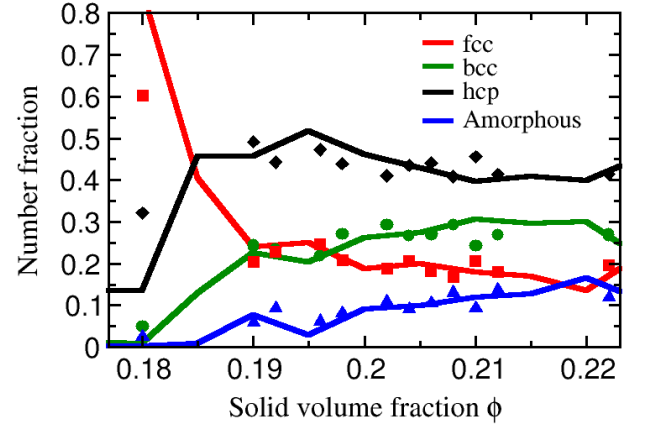

FIG. S5. Number fraction of the phases found in the simulations as a function of the particle volume fraction for the TM50 dispersion equilibrated with a bulk solution containing 5 mM of a monovalent salt at pH 9. Full lines give the results obtained with  $N = 19991$  particles, while the symbols those with  $N = 4009$ .

better approximation of the phase diagram might be ob-

tained by thermodynamic integration combined with the corrected equation of state, S7, derived by Boon et al. [6]. However, this method would be incapable of determining the truly thermodynamic phase behavior in the region of the observed glass-forming liquid. In principle, the semi-grand isobaric ensemble developed by Wilding et al. [14] could solve these issues. This method is nonetheless complicated by the density and composition dependence of the effective pair potentials. This is not only a question of technical difficulties. Indeed, in the thermodynamic limit, relevant when one is interested in computing/determining a phase diagram, each phase may have its own particle size distribution and density. The effective pair potentials would thus need to be computed for each specific density and composition visited during the course of the simulations, for example. Obviously, one can always disregard this problem, as has been done in the present work, where it seems to be a good approximation. However, when a high degree of fractionation is at work this approximation might break down, introducing inaccuracies into the phase diagram.

### S7. SIMULATION SNAPSHOTS AT PHASE COEXISTENCE

Two representative simulation snapshots of the TM50 dispersions, equilibrated with a solution containing 5 mM of salt and at pH 9, illustrating the phase coexistence in the dominant equilibrium domain of the fcc phase ( $\phi = 18.5\%$ ) and just after the fcc-bcc phase transition ( $\phi = 20.5\%$ ) are shown in Fig. S6. A stratified structure is observed when the hcp and fcc crystalline phases coexist. On the other hand, an intermixed structure between the hcp and bcc phase is found at higher volume fractions. This finding, together with the obtained ramified texture (as best illustrated by the cluster analysis given in Table I), suggests a spinodal decomposition of the dispersion, or at least that the interfacial free energy between the two phases is very low.

The particles in fcc arrangements, on the other hand, form many small and independent crystals, as detailed in Table I. The fluid particles are essentially located at the interface between the hcp and fcc or the bcc and fcc domains but not between the hcp and bcc phases. This further indicates that the surface tension of the hcp and bcc phases is very small and that of the fcc crystals is comparatively high.

### S8. PHASE COMPOSITION AND POLYDISPERSITY

Details of the polydispersity of the particles within individual phases, and at different  $\phi$ , are shown in Fig. S7. There is a slight fractionation of particles, increasing with  $\phi$ . As the crystal phases exclude certain particles at the extreme ends of the particle size distribution, the

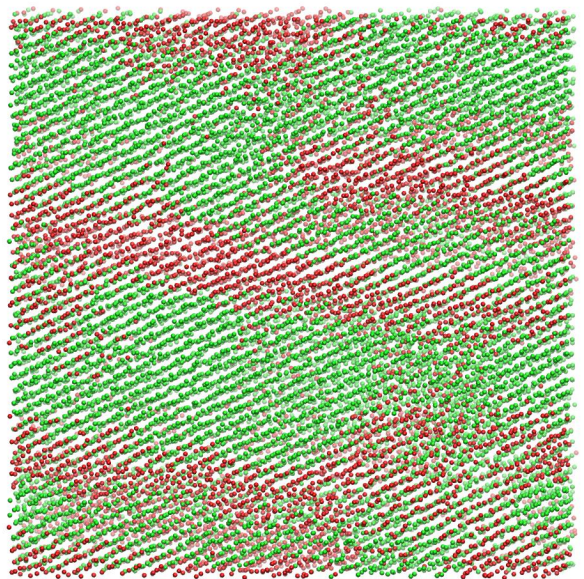

(a)

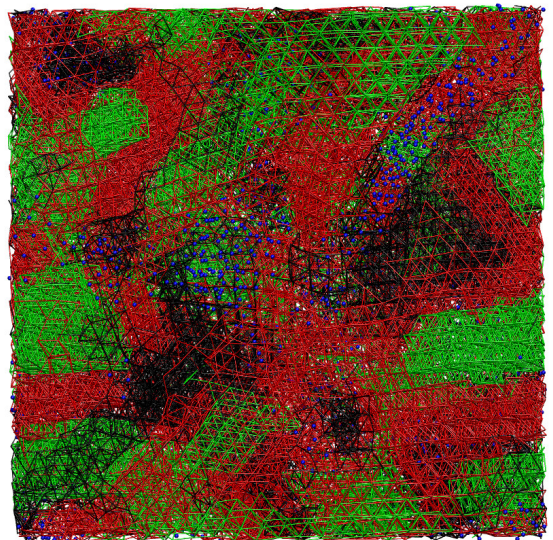

(b)

FIG. S6. Simulation snapshots at (a)  $\phi = 0.185$  and (b)  $\phi = 0.205$  of the TM50 dispersion equilibrated with a bulk solution containing 5 mM of a monovalent salt at pH 9. The same colors as in Fig. S4 are used, that is black for the bcc phase, red for the hcp phase, green for fcc phase and blue for the fluid phase. The simulations are performed with  $N = 19991$ . The cubic box side lengths are equal to 1059.9 nm and 1025 nm in (a) and (b), respectively.

TABLE I. Solid phase analysis of equilibrated TM50 silica suspension at  $\phi = 20.5\%$  pH 9 and  $c_s = 5\text{mM}$  as obtained for two different system sizes ( $N$ ). The analysis is here limited to one snapshot. A cluster analysis is used to determine the size of the largest cluster.

| Phase $i$ | $N = 40009$ |                              | $N = 19991$ |                              |
|-----------|-------------|------------------------------|-------------|------------------------------|
|           | $N_i^a$     | largest cluster <sup>b</sup> | $N_i^a$     | largest cluster <sup>b</sup> |
| bcc       | 10476       | 10266(0.98)                  | 5100        | 5049(0.99)                   |
| hcp       | 17991       | 17980(0.999)                 | 8704        | 8694(0.999)                  |
| fcc       | 8335        | 2144(0.26)                   | 4533        | 1230(0.27)                   |

<sup>a</sup>  $N_i$  gives the number of particles belonging to phase  $i$ .

<sup>b</sup> The largest cluster of the phase  $i$  is defined by the number of particles to which they belongs. Bracketed values give the corresponding number fraction.

polydispersity of the coexisting liquid phase increases as that of the crystal phases decreases.

Furthermore, for one set of experimental conditions, at pH9,  $c_s = 5\text{ mM}$  and  $\phi = 0.22$ , we performed simulations by changing the polydispersity of the system. Experimentally, these conditions give rise to a coexistence between bcc and fcc phases here, and were shown previously [4] to have a coexistence between a  $\text{MnZn}_2$  Laves phase and a bcc phase, at higher  $\delta$ . The simulations, detailed in Fig. S8, accurately reproduce this shift in phase equilibrium.

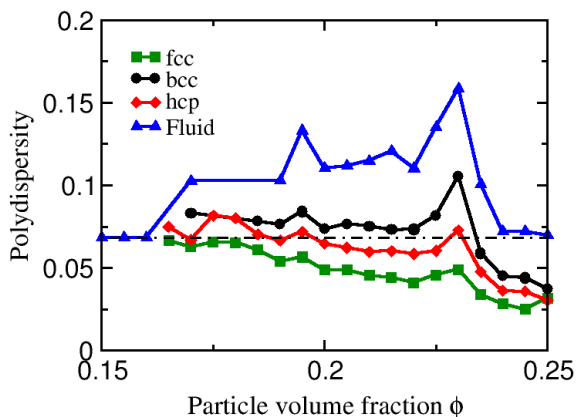

FIG. S7. Variation of the particle polydispersity in the various phases with the volume fraction of an aqueous silica dispersion at pH 9 and  $c_s = 5\text{ mM}$ . The polydispersity of the parent suspension is indicated by the dotted-dashed line. Jump in polydispersities is found at phase transitions. The particle polydispersity of the bcc phase is systematically higher than that of the fcc phase, showing that it is more tolerant of polydispersity.

## S9. LATTICE SIMULATION DESCRIPTION AND RESULTS

In order to better understand the mechanisms at play in the stabilization of the bcc solid phase in the polydis-

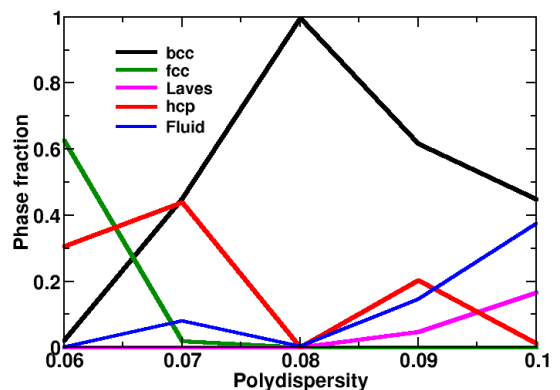

FIG. S8. Variation of the phase composition with the polydispersity (normal distribution) of an aqueous silica dispersion at pH 9,  $c_s = 5\text{ mM}$  and  $\phi = 22\%$ . Note the appearance of a  $\text{MgZn}_2$  Laves phase for polydispersities larger than 8%. The simulations were performed with 4000 particles.

perse TM50 silica dispersion at high salt concentrations and volume fractions we also performed simple lattice simulations, identical to that used in our previous studies [4, 15]. In short, the lattice simulations are performed in the Gibbs ensemble with 40000 particles assuming the coexistence between the bcc and fcc lattice structures. For simplicity, the hcp phase was not considered here. The system consists of two simulation boxes, one with a bcc lattice and one with a fcc lattice, each filled with a predefined number of particles randomly distributed over the lattice sites. The simulation boxes are allowed to change their volume while keeping the total system volume constant. Pairs of particles can swap their lattice positions if they belong either to the same or to a different box. The number of particles/lattices per box are, however, not allowed to change during the course of a simulation. Instead, separate simulations are performed with various pre-set fraction of bcc particles/sites,  $x_{bcc} = N_{bcc}/N_{tot}$ , but keeping the same total number of particles/sites,  $N_{tot} = N_{bcc} + N_{fcc}$ .

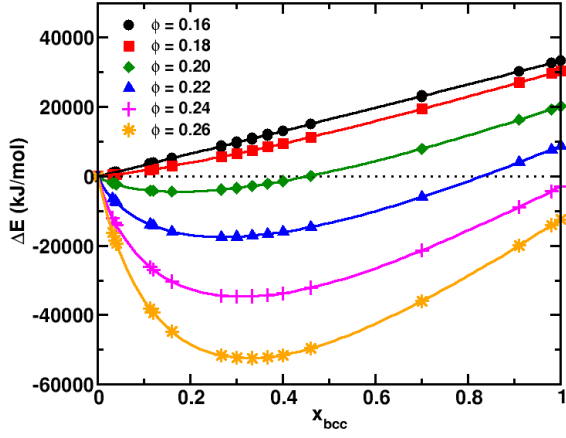

(a)

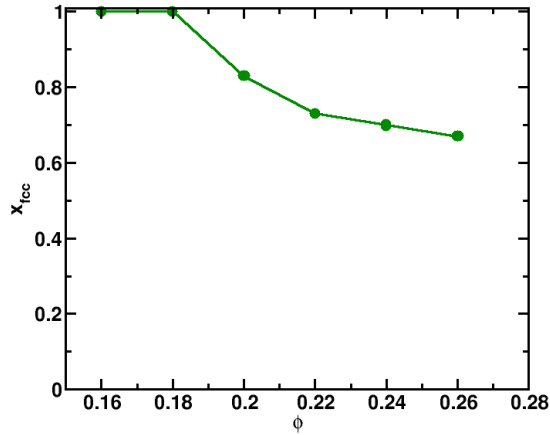

(b)

FIG. S9. Lattice simulation results of the difference in the total system energy,  $\Delta E$ , between a system constituted of only one fcc solid phase  $x_{bcc} = 0$  and a system made of the coexistence of bcc and fcc lattice structures varying the fraction of particles in the bcc lattice structure,  $x_{bcc}$ , at various particle volume fraction,  $\phi$ . Negative values of  $\Delta E$  indicate that the two solid phases in coexistence are more stable than a pure fcc structure. (b) Variation of the particle fraction in the fcc solid phase at equilibrium as a function of  $\phi$ . The equilibrium is approximated here as being the minimum in the total system energy (or equivalently the minimum in  $\Delta E$ ).

The difference in the total system energy when varying the fraction of bcc particles,  $x_{bcc}$ , at various (total) particle volume fractions is shown in Fig. S9. Note that the salt concentration is set to 5 mM and the pH to 9. Similarly to the continuous simulations, the proportion of particles in the bcc lattice is found to increase with increasing the volume fraction. Interestingly enough, the volume fraction where the particles start to fill the bcc lattice is found to be very near to that for which a stable bcc solid phase start to form in the continuous simulations. Though, their proportion is somewhat lower (com-

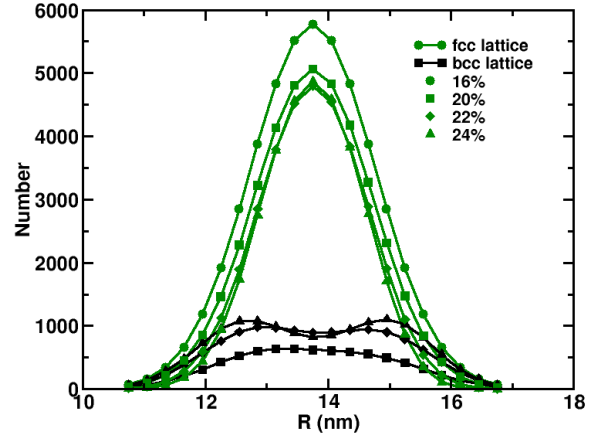

(a)

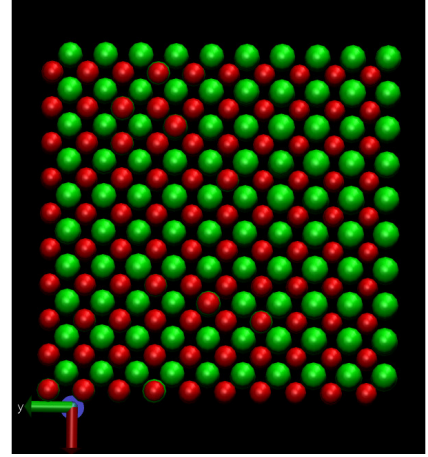

(b)

FIG. S10. (a) Variation of the particle size distribution in the bcc lattice and fcc lattice with  $\phi$  as obtained with the lattice simulations. (b) Simulation snapshot of the simulation box defined with a bcc lattice at  $\phi = 0.24$ ,  $c_s = 5\text{mM}$  and pH 9.

pare Figure S9(b) and Fig. 4 of the main manuscript). Also, in good agreement with the continuous simulations the particle fractionation between the two solid phases is found to be limited as illustrated by their particle distributions plotted in Fig. S10(a).

A clear distinction is obtained, however, when one compares the shape of the particle size distributions. Contrary to the continuous simulations and the experiments, the particles in the bcc lattice present a bimodal distribution, see Fig. S10(a). This is explained by the formation of a CsCl superlattice as it can be clearly seen in the simulation snapshot shown in Fig. S10(b).

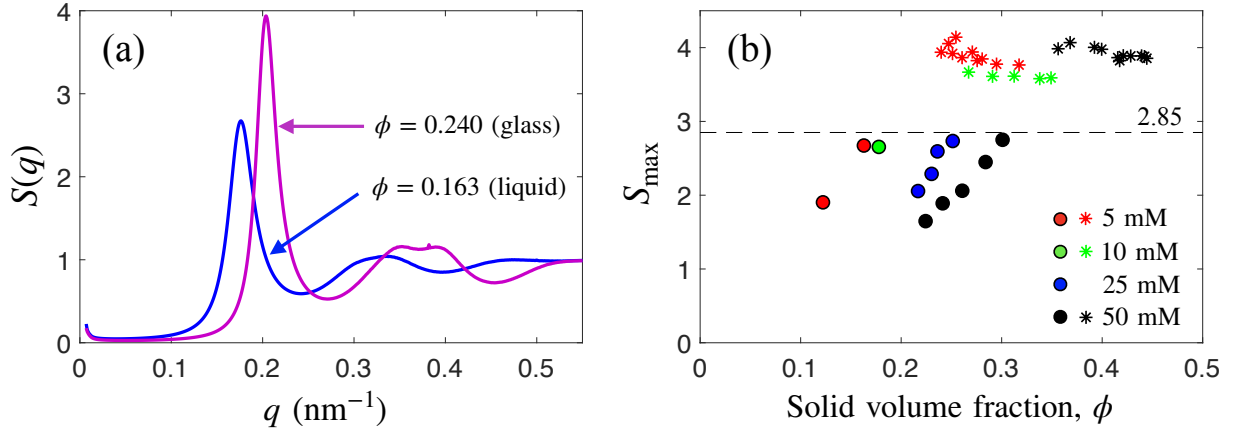

FIG. S11. Experimental observations of the amorphous phases. (a) The structure factor  $S(q)$  is shown for (i) a colloidal liquid, just below the volume fraction at which crystals were seen and (ii) the re-entrant amorphous phase, just above the last volume fraction at which crystals were seen (data for  $c_s = 5$  mM). (b) The maximum height of the structure factor,  $S_{\max}$  is known to characterise the stability of a colloidal liquid. Data are shown here for the low- $\phi$  liquid phase (circles) and high- $\phi$  glass phase (stars). Colloidal crystals are seen at the intermediate volume fractions. Their first appearance is consistent with the Verlet-Hansen criterion, shown as a dashed line.

### S10. CHARACTERISATION OF LIQUID AND GLASS PHASES

To experimentally characterise the structure of the liquid and glass phases, we calculated the structure factor  $S(q)$  by taking the ratio of the scattering intensity  $I(q)$  and a corresponding form factor measured in the dilute limit where  $\phi = 0.1\%$ . The results were normalised so that  $S(q) = 1$  at high  $q$ . Example structure factors for dispersions of 5 mM NaCl are given in Fig. S11(a). At all salt concentrations studied, the first appearance of crystals agreed with the Verlet-Hansen criterion [16, 17], which states that the liquid phase should be unstable when the maximum value of the structure factor,  $S_{\max}$  exceeds 2.85 (Fig. S11(b)). The high- $\phi$  glass phase consistently has a higher  $S_{\max}$ . The second peak of the glassy structure factor is also split, as demonstrated in Fig. S11(a).

For our simulations, Fig. S12 provides the coordination number (CN) of the particles in the fluid and glass forming liquid at pH 9, for  $c_s = 5$  mM (note that other salt concentrations give very similar results). The CN is defined as the number of particles within a cut-off radius taken as the first minimum of the radial distribution function. For the low- $\phi$  fluid phase, the coordination number is found to be rather constant, with  $\text{CN} = 13.2 \pm 0.02$  above  $\phi \approx 10\%$ , which can be viewed as the threshold value that delimits the diluted from the semi-diluted regime. This threshold increases with  $c_s$  and pH. The  $\text{CN} = 13 \pm 0.02$  of particles in the glassy phase is also rather constant and is nearly identical to that observed in the fluid phase, though slightly lower. A local structure analysis well inside the glassy phase reveals particles with icosahedral packing, which are virtually absent in

the equilibrium fluid phase. Those particles are charac-

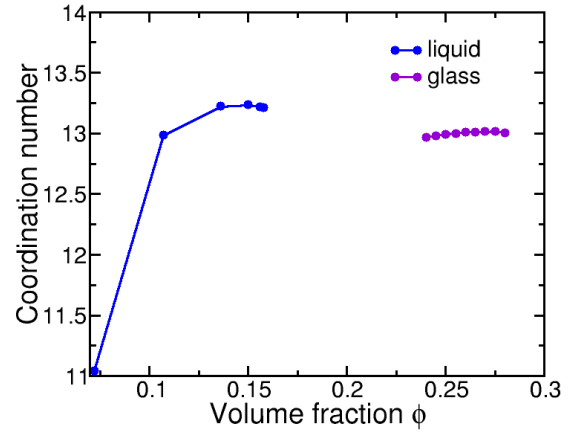

FIG. S12. Average coordination number of the particles in the fluid and glass forming liquid as obtained from MC simulations of aqueous TM50 silica dispersions at pH 9 and  $c_s = 5$  mM. The discontinuity in the curve corresponds to the solid phase region where not a good statistic for the CN of fluid particles could be obtained mainly because they are located at the interface between solid crystals.

terized by a high  $q_6$  and low  $q_4$  values (local bond order parameters) as well as a negative crystallinity factor, as defined by Leocmach, Russo and Tanaka [18]. A non-negligible fraction of particles ( $\approx 10\%$ ) are part of an icosahedral motif, similar to polydisperse hard sphere glass formers [19]. This local structuring of the particles is thought to be responsible for the high  $S_{\max}$  values and doubling of the second peak observed in the structure factor depicted in Fig. S11.

- 
- [1] Robert Botet and Bernard Cabane, “Simple inversion formula for the small-angle X-ray scattering intensity from polydisperse systems of spheres,” *J. Appl. Crystallogr.* **45**, 406–416 (2012).
  - [2] Verena Goertz, Nico Dingenouts, and Hermann Nirschl, “Comparison of Nanometric Particle Size Distributions as Determined by SAXS, TEM and Analytical Ultracentrifuge,” *Part. Part. Syst. Charact.* **26**, 17–24 (2009).
  - [3] Joaquim Li, Bernard Cabane, Michael Sztucki, Jérémie Gummel, and Lucas Goehring, “Drying Dip-Coated Colloidal Films,” *Langmuir* **28**, 200–208 (2012).
  - [4] Bernard Cabane, Joaquim Li, Franck Artzner, Robert Botet, Christophe Labbez, Guillaume Bareigts, Michael Sztucki, and Lucas Goehring, “Hiding in Plain View: Colloidal Self-Assembly from Polydisperse Populations,” *Phys. Rev. Lett.* **116**, 208001 (2016).
  - [5] Guillaume Bareigts and Christophe Labbez, “Jellium and cell model for titratable colloids with continuous size distribution,” *J. Chem. Phys.* **149**, 244903 (2018).
  - [6] Niels Boon, Guillermo Ivan Guerrero-García, René van Roij, and Monica Olvera de la Cruz, “Effective charges and virial pressure of concentrated macroion solutions,” *PNAS* **112**, 9242–9246 (2015).
  - [7] G. H. Bolt, “Determination of the Charge Density of Silica Sols,” *J. Phys. Chem.* **61**, 1166–1169 (1957).
  - [8] Christophe Labbez, Bo Jonsson, Michal Skarba, and Michal Borkovec, “Ion-ion correlation and charge reversal at titrating solid interfaces,” *Langmuir* **25**, 7209–7213 (2009).
  - [9] P. M. Dove and C. M. Craven, “Surface charge density on silica in alkali and alkaline earth chloride electrolyte solutions,” *Geochim Cosmochim. Acta* **69**, 4963–4970 (2005).
  - [10] Tomás S. Grigera and Giorgio Parisi, “Fast Monte Carlo algorithm for supercooled soft spheres,” *Phys. Rev. E* **63**, 045102 (2001).
  - [11] Carolina Brito, Edan Lerner, and Matthieu Wyart, “Theory for Swap Acceleration near the Glass and Jamming Transitions for Continuously Polydisperse Particles,” *Phys. Rev. X* **8**, 031050 (2018).
  - [12] D. Frenkel and B. Smit, *Understanding Molecular Simulation* (Academic Press, San Diego, 2002).
  - [13] Wolfgang Lechner and Christoph Dellago, “Accurate determination of crystal structures based on averaged local bond order parameters,” *The Journal of Chemical Physics* **129**, 114707 (2008).
  - [14] Nigel B. Wilding and Peter Sollich, “Phase behavior of polydisperse spheres: Simulation strategies and an application to the freezing transition,” *The Journal of Chemical Physics* **133**, 224102 (2010).
  - [15] Robert Botet, Bernard Cabane, Lucas Goehring, Joaquim Li, and Franck Artzner, “How do polydisperse repulsive colloids crystallize?” *Faraday Discuss.* **186**, 229–240 (2016).
  - [16] Loup Verlet, “Computer Experiments on Classical Fluids. II. Equilibrium Correlation Functions,” *Phys. Rev.* **165**, 201–214 (1968).
  - [17] Jean-Pierre Hansen and Loup Verlet, “Phase Transitions of the Lennard-Jones System,” *Phys. Rev.* **184**, 151–161 (1969).
  - [18] Mathieu Leocmach, John Russo, and Hajime Tanaka, “Importance of many-body correlations in glass transition: An example from polydisperse hard spheres,” *The Journal of Chemical Physics* **138**, 12A536 (2013).
  - [19] Daniele Coslovich, Misaki Ozawa, and Ludovic Berthier, “Local order and crystallization of dense polydisperse hard spheres,” *J. Phys.: Condens. Matter* **30**, 144004 (2018).
